# Supplementary material for: Improving Semantic Control in Discrete Latent Spaces with Transformer Quantized Variational Autoencoders
Source: arXiv:2402.00723 source file (2024-02-01)
Supplement: Supplementary file 1 [file appendix_sub_traversal.tex]

% traversals results
\begin{table}[ht!]
\begin{tcolorbox}[fontupper=\small, fontlower=\small, title=Traversal with different premise]
\textbf{\underline{P2: flowing can be a kind of transfer of energy}} \\
\begin{multicols}{2}
P1: \textcolor{blue}{heat} is a kind of energy \\
P1: \textcolor{blue}{heat} is energy \\
P1: \textcolor{blue}{heat} means energy \\
P1: \textcolor{blue}{heat} = energy \\
P1: energy can be \textcolor{blue}{heat} \\
P1: energy includes \textcolor{blue}{heat} \\
P1: \textcolor{blue}{water} is a kind of energy \\

\columnbreak
\\ \\ \\

Pred: flowing can be a kind of transfer of \textcolor{blue}{heat} \\
Pred: flowing can be a kind of transfer of \textcolor{blue}{heat} \\
Pred: flowing can be a kind of transfer of \textcolor{blue}{heat} \\
Pred: flowing can be a kind of transfer of \textcolor{blue}{heat} \\
Pred: flowing can be a kind of transfer of \textcolor{blue}{heat} \\
Pred: flowing can be a kind of transfer of \textcolor{blue}{heat} \\
Pred: flowing can be a kind of transfer of \textcolor{blue}{water} \\
\end{multicols}
\end{tcolorbox}
\caption{T5VQVAE(base): traversal with various premise.}
\label{tab:appendix_quasi}
\end{table}
